# Supplementary material for: Predicting Water Temperature Dynamics of Unmonitored Lakes with Meta Transfer Learning
Source: arXiv:2011.05369 source file (2021-06-17)
Supplement: Supplementary file 1 [file si_template_2019.tex]

% %%%%%%%%%%%%%%%%%%%%%%%%%%%%%%%%%%%%%%%%%%%%%%%%%%%%%%%%%%%%%%%%%%%%%%%%%%%%
% % AGUtmpl.tex: this template file is for articles formatted with LaTeX2e,
% % Modified December 2018
% %
% % This template includes commands and instructions
% % given in the order necessary to produce a final output that will
% % satisfy AGU requirements.
% %
% % FOR FIGURES, DO NOT USE \psfrag
% %
% %%%%%%%%%%%%%%%%%%%%%%%%%%%%%%%%%%%%%%%%%%%%%%%%%%%%%%%%%%%%%%%%%%%%%%%%%%%%
% %
% % IMPORTANT NOTE:
% %
% % SUPPORTING INFORMATION DOCUMENTATION IS NOT COPYEDITED BEFORE PUBLICATION.
% %
% %
% %
% %%%%%%%%%%%%%%%%%%%%%%%%%%%%%%%%%%%%%%%%%%%%%%%%%%%%%%%%%%%%%%%%%%%%%%%%%%%%
% %
% % Step 1: Set the \documentclass
% %
% %
% % PLEASE USE THE DRAFT OPTION TO SUBMIT YOUR PAPERS.
% % The draft option produces double spaced output.
% %
% % Choose the journal abbreviation for the journal you are
% % submitting to:

% % jgrga JOURNAL OF GEOPHYSICAL RESEARCH (use for all of them)
% % gbc   GLOBAL BIOCHEMICAL CYCLES
% % grl   GEOPHYSICAL RESEARCH LETTERS
% % pal   PALEOCEANOGRAPHY
% % ras   RADIO SCIENCE
% % rog   REVIEWS OF GEOPHYSICS
% % tec   TECTONICS
% % wrr   WATER RESOURCES RESEARCH
% % gc    GEOCHEMISTRY, GEOPHYSICS, GEOSYSTEMS
% % sw    SPACE WEATHER
% % ms    JAMES
% % ef    EARTH'S FUTURE
% %
% %
% %
% % (If you are submitting to a journal other than jgrga,
% % substitute the initials of the journal for "jgrga" below.)

% \documentclass[draft,wrr]{agutexSI2019}

% %%%%%%%%%%%%%%%%%%%%%%%%%%%%%%%%%%%%%%%%%%%%%%%%%%%%%%%%%%%%%%%%%%%%%%%%%
% %
% %  SUPPORTING INFORMATION TEMPLATE
% %
% %% ------------------------------------------------------------------------ %%
% %
% %
% %Please use this template when formatting and submitting your Supporting Information.

% %This template serves as both a “table of contents” for the supporting information for your article and as a summary of files.
% %
% %
% %OVERVIEW
% %
% %Please note that all supporting information will be peer reviewed with your manuscript. It will not be copyedited if the paper is accepted.
% %In general, the purpose of the supporting information is to enable authors to provide and archive auxiliary information such as data tables, method information, figures, video, or computer software, in digital formats so that other scientists can use it.
% %The key criteria are that the data:
% % 1. supplement the main scientific conclusions of the paper but are not essential to the conclusions (with the exception of
% %    including %data so the experiment can be reproducible);
% % 2. are likely to be usable or used by other scientists working in the field;
% % 3. are described with sufficient precision that other scientists can understand them, and
% % 4. are not exe files.
% %
% %USING THIS TEMPLATE
% %
% %***All references should be included in the reference list of the main paper so that they can be indexed, linked, and counted as citations.  The reference section does not count toward length limits.
% %
% %All Supporting text and figures should be included in this document. Insert supporting information content into each appropriate section of the template. To add additional captions, simply copy and paste each sample as needed.


% %IMPORTANT NOTE ON FIGURES AND TABLES
% % Placeholders for figures and tables appear after the \end{article} command, after references.
% % DO NOT USE \psfrag or \subfigure commands.
% %
% \usepackage{graphicx}
% \usepackage{url} %this package should fix any errors with URLs in refs.
% \usepackage{lineno}
% \usepackage[inline]{trackchanges} %for better track changes. finalnew option will compile document with changes incorporated.
% \usepackage{soul}
% \usepackage{siunitx}
% \sisetup{output-exponent-marker=\ensuremath{\mathrm{e}}}
% \linenumbers
% \newcommand{\NA}{---}
% \draftfalse
% \usepackage{multirow}
% \usepackage{amssymb}
% \usepackage{xcolor}
% % \usepackage{float}
% \usepackage{gensymb}
% \usepackage{textcomp}
% \usepackage{amsmath}
% \usepackage{graphicx}
% \usepackage{array}
% \usepackage{booktabs}
% \usepackage{longtable}
% \usepackage{caption}
% \usepackage{subcaption}
% \usepackage{placeins}
% \usepackage{threeparttable}
% \newcommand{\yell}[1]{{\color{red} \textbf{#1}}}
% \usepackage{makecell}
% \renewcommand\theadalign{ll}
% \renewcommand\theadfont{}
% \renewcommand\theadgape{\Gape[4pt]}%
% %  Uncomment the following command to allow illustrations to print
% %   when using Draft:
% \setkeys{Gin}{draft=false}
% %
% % \makeatletter
% % \renewcommand \thefigure {\@arabic\c@figure}
% % \def\fps@figure{tbp}
% % \def\ftype@figure{1}
% % \def\ext@figure{lof}
% % \def\fnum@figure{Figure\nobreakspace\thefigure}
% % \newenvironment{figure}{\@float{figure}}{\end@float}
% % \makeatother
% % You may need to use one of these options for graphicx depending on the driver program you are using. 
% %
% % [xdvi], [dvipdf], [dvipsone], [dviwindo], [emtex], [dviwin],
% % [pctexps],  [pctexwin],  [pctexhp],  [pctex32], [truetex], [tcidvi],
% % [oztex], [textures]
% %
% %
% %% ------------------------------------------------------------------------ %%
% %
% %  ENTER PREAMBLE
% %
% %% ------------------------------------------------------------------------ %%

% % Author names in capital letters:
% %\authorrunninghead{BALES ET AL.}

% % Shorter version of title entered in capital letters:
% %\titlerunninghead{SHORT TITLE}
% %Corresponding author mailing address and e-mail address:
% %\authoraddr{Corresponding author: A. B. Smith,
% %Department of Hydrology and Water Resources, University of
% %Arizona, Harshbarger Building 11, Tucson, AZ 85721, USA.
% %(a.b.smith@hwr.arizona.edu)}
% \usepackage{xr}
% \makeatletter
% \newcommand*{\addFileDependency}[1]{
%   \typeout{(#1)}
%   \@addtofilelist{#1}
%   \IfFileExists{#1}{}{\typeout{No file #1.}}
% }
% \makeatother

% \newcommand*{\myexternaldocument}[1]{
%     \externaldocument{#1}
%     \addFileDependency{#1.tex}
%     \addFileDependency{#1.aux}
% }

% \myexternaldocument{agu_journal_main_text}
% % %%%%%%%%%% Merge with supplemental materials %%%%%%%%%%
% % %%%%%%%%%% Prefix a "S" to all equations, figures, tables and reset the counter %%%%%%%%%%
% \setcounter{equation}{0}
% \setcounter{figure}{0}
% \setcounter{table}{0}
% \setcounter{page}{1}
% \makeatletter
% \renewcommand{\theequation}{S\arabic{equation}}
% \renewcommand{\thefigure}{S\arabic{figure}}
% \setcounter{section}{0}
% \renewcommand{\thesection}{S\Roman{section}}



% %% ------------------------------------------------------------------------ %%
% %
% %  TITLE
% %
% %% ------------------------------------------------------------------------ %%

% %\includegraphics{agu_pubart-white_reduced.eps}



% %
% % e.g., \title{Supporting Information for "Terrestrial ring current:
% % Origin, formation, and decay $\alpha\beta\Gamma\Delta$"}
% %
% %DOI: 10.1002/%insert paper number here%

% %% ------------------------------------------------------------------------ %%
% %
% %  AUTHORS AND AFFILIATIONS
% %
% %% ------------------------------------------------------------------------ %%


% % List authors by first name or initial followed by last name and
% % separated by commas. Use \affil{} to number affiliations, and
% % \thanks{} for author notes.
% % Additional author notes should be indicated with \thanks{} (for
% % example, for current addresses).

% % Example: \authors{A. B. Author\affil{1}\thanks{Current address, Antartica}, B. C. Author\affil{2,3}, and D. E.
% % Author\affil{3,4}\thanks{Also funded by Monsanto.}}

% \begin{document}
% \title{Supporting Information for "Predicting Water Temperature Dynamics of Unmonitored Lakes with Meta Transfer Learning"}
% \authors{
% Jared D. Willard\affil{1,2} , Jordan S. Read\affil{2}, Alison P. Appling\affil{2}, Samantha K. Oliver\affil{2}, Xiaowei Jia\affil{3}, and Vipin Kumar\affil{1}}

% \affiliation{1}{Department of Computer Science and Engineering, University of Minnesota, Minneapolis, MN, USA}
% \affiliation{2}{U.S. Geological Survey, Middleton, WI, USA
% }
% \affiliation{3}{Department of Computer Science, University of Pittsburgh, Pittsburgh, PA, USA}
% % \affiliation{1}{First Affiliation}
% % \affiliation{2}{Second Affiliation}
% % \affiliation{3}{Third Affiliation}
% % \affiliation{4}{Fourth Affiliation}

% % \affiliation{=number=}{=Affiliation Address=}
% %(repeat as many times as is necessary)





% %% ------------------------------------------------------------------------ %%
% %
% %  BEGIN ARTICLE
% %
% %% ------------------------------------------------------------------------ %%

% % The body of the article must start with a \begin{article} command
% %
% % \end{article} must follow the references section, before the figures
% %  and tables.

% \begin{article}

% %% ------------------------------------------------------------------------ %%
% %
% %  TEXT
% %
% %% ------------------------------------------------------------------------ %%



% \noindent\textbf{Contents of this file}
% %%%Remove or add items as needed%%%
% \begin{enumerate}
% \item Text S1 to Sx
% \item Figures S1 to Sx
% \item Tables S1 to Sx
% %if Tables are larger than 1 page, upload as separate excel file
% \end{enumerate}
% \noindent\textbf{Additional Supporting Information (Files uploaded separately)}
% \begin{enumerate}
% \item Captions for Datasets S1 to Sx
% \item Captions for large Tables S1 to Sx (if larger than 1 page, upload as separate excel file)
% \item Captions for Movies S1 to Sx
% \item Captions for Audio S1 to Sx
% \end{enumerate}

% \noindent\textbf{Introduction}
% %Type or paste your text here. The introduction gives a brief overview of the supporting information. You should include information %about as many of the following as possible (when appropriate):
% % 1. a general overview of the kind of data files;
% % 2. information about when and how the data were collected or created;
% % 3. a general description of processing steps used;
% % 4. any known imperfections or anomalies in the data.

% %\clearpage

% %Delete all unused file types below. Copy/paste for multiples of each file type as needed.
% \noindent\textbf{Text S1.}
% \label{supp:pgdl}
% \subsection{Physics-Guided Deep Learning Model Details}
% \subsubsection{Input Features}
% Input features were shown in Table \ref{tab:input} and described in Section \ref{method-pgdl}. Prior to being used by the model, z-score normalization to a mean 0 and standard deviation 1 was performed to put all input features on the same scale \cite{patro2015normalization}. An unscaled version of the features was also kept to calculate the process-based energy conservation loss term, as described in the following subsection.

% \subsubsection{Long Short Term Memory (LSTM) Model}
% LSTM neural networks \cite{hochreiter1997long} are a variant of the recurrent neural network, the most widely used deep learning architecture for temporal sequence modeling. They form the basis for these PGDL models. The power of the LSTM model lies in its ability to combine inputs at both the current and many previous time steps into "memories", or hidden state values that the LSTM selectively retains from one timestep to the next. In this lake temperature application, such memories might represent short-term history such as recent water temperatures, and long-term processes such as thermocline movement, changes in stratification, layer mixing over time, and gradual freezing and melting.

% \subsubsection{Process-Based Loss Function Terms}
% Loss function terms optimizing for physical consistency address a known drawback in machine learning applications to physical systems, which is that output is not guaranteed to conform to known physical laws \cite{karpatne2017physics, karpatne2017theory}. In this this work we use two additional loss terms, an energy consistency loss and a density-depth consistency loss. 

% In conjunction with the standard mean squared error loss term for regression, the energy consistency loss term \cite{jia2019physics, read2019process} was used to weakly constrain the network output to conform to the law of conservation of energy. Conservation of energy is a first principle implemented in GLM and other similar process-based models: The volume-averaged change in lake thermal energy (dU) should match the net energy flux over the same time period (dt). The net flux can be calculated in units $W/m^2$ as 

% \begin{equation}
% \small
%     \frac{dU}{dt} = \Phi_{SW_{in}} - \Phi_{E} - \Phi_{H} + \Phi_{LW_{in}} - \Phi_{LW_{out}}
% \end{equation}

% where $\Phi_{SW_{in}}$ is the incoming shortwave radiation minus a fraction reflected (7\%), $\Phi_{E}$ and $\Phi_{H}$ are the latent and sensible heat fluxes, $\Phi_{LW_{in}}$ is the incoming longwave radiation minus a fraction reflected (3\%), and $\Phi_{LW_{out}}$ is the longwave radiation emitted from the lake. All these terms can be calculated from the input drivers in Table~\ref{tab:input} and the predicted surface temperature, details of which are given in \cite{jia2019physics, hipsey2019general}. 

% The thermal energy at any point in time can then be estimated based on water temperatures and horizontal cross-sectional area at each depth:

% \begin{equation}
% \small
%     U = \frac{c_w}{A_s}\sum_{i=1}^{n_{layers}}\rho_{i}T_{i}V_{i}
% \end{equation}

% where $c_w$ is the specific heat capacity of water (4186 J kg\textsuperscript{-1}  \degree C\textsuperscript{-1}),  A\textsubscript{s} is the  surface area of the lake (in m\textsuperscript{2}), $\rho$\textsubscript{i} is the water density (kg m\textsuperscript{-3}), T\textsubscript{i} is the water temperature (\textdegree C), and V\textsubscript{i} is the volume (in m\textsuperscript{3}), all for each depth layer $i$ of the model. Furthermore, since these equations hold only when the lake is not ice covered, we limit our loss term to only the ice-free time steps as determined by the GLM predictions of ice cover. We also include a term $\tau_{\text{EC}}$ that thresholds the value to account for simplification in the flux calculation and observation error in the meteorological drivers or bathymatric maps. The loss term can then be written as
 
%  \begin{equation}
% \small
%     \text{Energy.Loss}(\hat{Y}) = \frac{1}{T_{\text{ice-free}}}\sum_{t \in \text{ice-free}} \text{ReLU}(|\Delta U_t - \frac{dU}{dT}| - \tau_{\text{EC}})
% \end{equation}


% In addition to the energy conservation loss function term, we incorporate a second physics-based term that penalizes the model for violating density consistency across the water column as is described in \cite{karpatne2017physics}. The density of water monotonically increases with depth, and this is implicitly encoded in process-based models. By constructing an additional loss term penalizing the neural network for violations of this basic physical principle, we can guide the model toward density-consistent solutions. Given the mapping from water temperature to density, the loss function term can be calculated on model outputs $\hat{Y}$ as the mean of all violations across every consecutive depth-pair and time-step:


% \begin{equation}
% \small
%     \text{Density.Loss}(\hat{Y}) = \frac{1}{n_t(n_d - 1)}\sum_{t=1}^{n_t}\sum_{i=1}^{n_d-1}\text{ReLU}(\hat{\rho}_{d_i,t} - \hat{\rho}_{d_{i+1,t}})
%     % Density.Loss(\hat{Y}) = \frac{1}{n_t(n_d - 1)}\sum_{t=1}^{n_t}\sum_{i=1}^{n_d-1}\text{ReLU}(\Delta [i,t])
% \end{equation}

% Here, $n_t$ is the number of timesteps, $n_d$ is the number of depths, and $\hat{\rho}_{d_i,t}$ is the density at a given depth and timestep. The total loss function then includes both the standard mean squared error loss for neural network regression and hyperparameters $\lambda_{\text{EC}}$ and $\lambda_{\text{DC}}$ for the magnitude of each physics-based term. 

% \begin{equation}
% \small
%     \text{Train.Loss} = \text{MSE}(Y, \hat{Y}) + \lambda_{\text{EC}}* \text{Energy.Loss}(\hat{Y}) + \lambda_{\text{DC}} *\text{Density.Loss}(\hat{Y})
% \end{equation}

% A visual representation of the information flow through the PGDL model is shown in Figure \ref{fig:pgrnn-dia}.
% %Type or paste text here. This should be additional explanatory text, such as: extended descriptions of results, full details of models, extended lists of acknowledgements etc.  It should not be additional discussion, analysis, interpretation or critique. It should not be an additional scientific experiment or paper.
% %
% %Repeat for any additional Supporting Text
% % \begin{figure}
% % \setfigurenum{S1} %%You can change number for each figure if you want, not required. "S" prepended automatically.
% % \noindent\includegraphics[natwidth=800px,natheight=600px]{doc/PGRNN_diag.png}
% % \caption{caption}
% % \label{epsfiguresample}
% % \end{figure}
% \begin{figure}[h]
% \setfigurenum{S1}
% \includegraphics[width=0.9\textwidth]{doc/PGRNN_diag.png}
% \caption{Information flow in the PGDL model. The model includes the standard RNN flow (black arrows) between  inputs and outputs at various time steps, the energy flow (blue arrows), and the density flow (orange arrows) in the recurrent process}
% \label{fig:pgrnn-dia}
% \end{figure}


% \subsubsection{Pre-training}
% Pre-training involves training the model on a separate dataset prior to the actual training. For the purpose of lake temperature prediction, we first train the PGDL model on process-based model simulation data. This allows for a more accurate and physically consistent initialized state for the LSTM to be further trained on actual observations. Simulation data was acquired from a parameterized but uncalibrated application of General Lake Model (GLM) v2.2 \cite{hipsey2019general} from the USGS data release ``Predicting Water Temperature Dynamics of Unmonitored Lakes with Meta Transfer Learning" \cite{willard2020data}. Both pre-training and additional loss function terms have been shown to improve learning performance and physical consistency in \cite{jia2019physics}. In the same study it was shown that pre-trained models can achieve high accuracy given only a few observed data points, a situation common in lake temperature modeling. 

% %  Among deep learning models, the recurrent neural network (RNN) is the most widely used for temporal sequence modeling. The power of the RNN model lies in its ability to combine inputs at both the current and previous time steps to extract informative hidden representations.

% % However, standard RNNs suffer from vanishing and exploding gradient problems that inhibit the flow of information from prior timesteps \cite{bengio1994learning}. LSTMs  deal with these problems by introducing new gates, called the input and forget gates, allowing for better control over the gradient flow and enable better preservation of long-range dependencies across time \cite{chung2014empirical}.


% \subsubsection{Hyperparameterization and Network Architecture}
% Based on prior PGDL work \cite{jia2019physics, read2019process}, each LSTM was trained with 20 hidden units in a single layer, one batch for all training data per epoch, and using sequences of 350 days of input drivers with observations spread throughout (though typically most common in the spring, summer, and fall). The initial weights of the model were samples from the Glorot normal distribution \cite{glorot2010understanding}. The 350 day window was shifted by 175 days to construct each input sequence to the model. Model output $\hat{Y}$ in the physics-informed terms of the loss function is a randomly selected 350 day sequence from the entire time period from training and testing data per epoch, since these terms does not require observations to be calculated. 

% The MSE loss is calculated only on days where observations took place in the second half of each sequence. This gives the network time to build memory of past drivers and observations prior to prediction. We note that even though the training loss is only defined at time steps where observations are available, the structure of the LSTM allows input drivers from all time steps to contribute to prediction during the training process. 

% Training is stopped when all three loss function terms converge for 10 epochs to the specified conditions of 
% \begin{enumerate}
%     \item Training Data $MSE(Y,\hat{Y}) < 1$
%     \item $\text{Energy.Loss}(\hat{Y}) < 40$
%     \item  $\text{Density.Loss}(\hat{Y}) < \begin{cases} .001,& \text{if pre-training} \\
%     .01 & \text{if training}\end{cases}$
% \end{enumerate}

% The two hyperparameters that weight the loss terms, \{$\lambda_{\text{EC}}$,$\lambda_{\text{DC}}$\}, were set to \{0.2, 10\} and \{.01, 2\} in the pre-training and training stages respectively, and $\tau_{\text{EC}}$ was set to 40 W/m\textsuperscript{2}. These values and conditions were  manually tuned to allow all loss terms to converge and therefore achieve training accuracy and physically consistent output across all lakes in the dataset. Since the PGDL source models are intended to be applied to target lakes \textit{without observations}, validation sets as usually defined in machine learning practice (e.g. using data separate from training and testing) may not be used to estimate generalizability for the given task. We therefore chose not to use validation error as a stopping condition for training, and instead opted for the conditions above.
% %-------------------------------------------------------------------
% \subsection{Additional Plots and Figures}


% %metamodel rank plot
% \clearpage
% \begin{figure}[H]
%     \centering
%     \includegraphics[width=\textwidth]{doc/metamodel_rankplot_PB.png}
%     \includegraphics[width=\textwidth]{doc/metamodel_rankplot_PG.png}
%     \caption{Plots visualizing the RMSEs of selected source PB models (top) and source PGDL models (bottom) compared to all possible sources. Red shows the top predicted PGDL model by the metamodel,  purple shows the top 9 predicted PGDL models, and gray shows the remaining sources}
%     \label{fig:meta_rankplot}
% \end{figure}


% %---------------------------------------------------
% \subsection{Visualizing Training Lakes (Source) and Test Lakes (Target)}
% \begin{figure}[H]
%   \centering
%     \includegraphics[width=\textwidth]{doc/train_test_scatter.png}
%   \caption{Visualization of the 145 training lakes and 305 test lakes in terms of two of the most important attributes included in the meta-features, maximum depth and surface area.}
%   \label{supp:fig:trn-tst-scatter}
% \end{figure}

% \subsection{Candidate Meta Features}

% \begin{table}
% \fontsize{7.5}{7.5}\selectfont
% \caption{\textit{Candidate Meta Feature Information}}
% \label{tab:metafeat}
% \begin{threeparttable}


% \begin{tabular}{|l|c|l|}
% \toprule
% \textbf{Meta Feature} & \textbf{Units} & \textbf{Additional Description} \\
% & & \\
% \midrule
% \thead{\textbf{Lake Attributes} \\\textbf{(Source/Target Differences)}}& & \\
% Difference in Max Depth & m & \\
% Percent Difference in Max Depth & percent & \\
% Difference in Surface Area & m\textsuperscript{2} & \\
% Percent Difference in Surface Area & percent & \\
% Difference in Square Root of Surface Area & m & \\
% \thead{Percent Difference in Square Root \\of Surface Area}& percent & \\
% Difference in Shoreline Development Factor & 1 & \\
% \thead{Difference in K\_d \\(Light Attenuation Coefficient)} & m\textsuperscript{-1} & \\
% Difference in Lathrop Stratification Index & 1 & 1 or 0 as defined in \cite{lathrop1980thermal}\\
% Difference in Latitude & degrees & \\
% Difference in Longitude & degrees & \\
% \midrule
% \textbf{Observation Statistics (Source Only)}& & \\
% Total Temperature Obs & samples & \\
% Total Sampling Dates & days/profiles & \\
% Number of Winter Obs & samples & Defined between solstice/equinox\\
% Number of Spring Obs & samples & Defined between solstice/equinox\\
% Number of Summer Obs & samples & Defined between solstice/equinox\\
% Number of Autumn Obs & samples & Defined between solstice/equinox\\
% \thead{Mean Depth of Obs \\as Fraction of Max Depth} & 1 & \\
% Mean Temp of Obs & deg C & \\
% \thead{Difference Between Average Observation \\ Temp and Average Air Temp} & deg C & \\
% Standard Deviation of Obs Temp & deg C & \\
% Skew of Obs Temp & 1 & \\
% Kurtosis of Obs Temp & 1 & \\
% \midrule
% \thead{\textbf{PB0 Simulation Statistics} \\\textbf{(Source/Target Differences)}}& & \\
% \thead{PB0 Stratification Period} & Percent & \thead{Difference in percentage of dates where \\temps differ more than 1°C in profile}\\

% \midrule
% \thead{\textbf{(Meteorological Statistics)}\\\textbf{(Source/Target Differences)}} & &  \\
% Shortwave Radiation & w/m\textsubscript{2} & \thead{10 Values - Difference in Mean/Std\_dev Total and Per Season} \\
% Longwave Radiation & w/m\textsubscript{2} & \thead{10 Values - Difference in Mean/Std\_dev Total and Per Season} \\
% Air Temp & deg C & \thead{10 Values - Difference in Mean/Std\_dev Total and Per Season} \\
% Air Temp Amplitude & deg C & Difference in Average Yearly Amplitude \\
% 0°C Day of Year & days & \thead{Difference in day of year (0-366) where first sequence of\\ 6 days with subzero temperatures begins}\\
% Relative Humidity & percent & \thead{10 Values - Difference in Mean/Std\_dev Total and Per Season}\\
% Wind Speed & m/s &\thead{10 Values - Difference in Mean/Std\_dev Total and Per Season}\\
% \thead{Wind Speeds During Spring Mixing Period} & m/s & \thead{Difference in 45 Day Average After 0\textdegree C Air Temp Estimate} \\
% Difference in Rain & m & \thead{10 Values - Mean/Std\_dev Total and Per Season}\\
% Difference in Snow & m & \thead{10 Values - Mean/Std\_dev Total and Per Season}\\
% \bottomrule
% \end{tabular}
% \begin{tablenotes}
% \item \normalsize\textit{Note}. Here, if $V_s$ is the source value and $V_t$ is the target value, then differences are defined as $V_s - V_t$, absolute differences as $|V_s - V_t|$, and percent differences as $\frac{|V_s - V_t|}{(V_t+V_s)/2}$.
% \end{tablenotes}

% \end{threeparttable}
% \end{table}


% \FloatBarrier
% \FloatBarrier
% \clearpage
% \newpage
% \bibliography{agu_journal_main_text} 
% % Information flow in the PGDL model. The model includes the standard RNN flow (black arrows) between  inputs and outputs at various time steps, the energy flow (blue arrows), and the density flow (orange arrows) in the recurrent process
% % \captionof{fig:pgrnn-dia}{your caption text}
% %%Enter Data Set, Movie, and Audio captions here
% %%EXAMPLE CAPTIONS

% % \noindent\textbf{Data Set S1.} %Type or paste caption here.
% % %upload your dataset(s) to AGU's journal submission site and select "Supporting Information (SI)" as the file type. Following naming %convention: ds01.

% % %Repeat for any additional Supporting data sets

% % \noindent\textbf{Movie S1.} %Type or paste caption here.
% % %upload your movie(s) to AGU's journal submission site and select, "Supporting Information %(SI)" as the file type. Following naming convention: ms01.

% % %Repeat any additional Supporting movies

% % \noindent\textbf{Audio S1.} %Type or paste caption here.
% % %upload your audio file(s) to AGU's journal submission site and select "Supporting Information %(SI)" as the file type. Following naming convention: auds01.


% %Repeat for any additional Supporting audio files

% %%% End of body of article:
% %%%%%%%%%%%%%%%%%%%%%%%%%%%%%%%%%%%%%%%%%%%%%%%%%%%%%%%%%%%%%%%%
% %
% % Optional Notation section goes here
% %
% % Notation -- End each entry with a period.
% % \begin{notation}
% % Term & definition.\\
% % Second term & second definition.\\
% % \end{notation}
% %%%%%%%%%%%%%%%%%%%%%%%%%%%%%%%%%%%%%%%%%%%%%%%%%%%%%%%%%%%%%%%%


% %% ------------------------------------------------------------------------ %%
% %%  REFERENCE LIST AND TEXT CITATIONS

% %%%%%%%%%%%%%%%%%%%%%%%%%%%%%%%%%%%%%%%%%%%%%%%
% % 
% %
% % \bibliography{<name of your .bib file>} do not specify file extension
% %
% % no need to specify bibliographystyle
% %
% % Note that ALL references in this supporting information file must also be referenced in the primary manuscript
% %
% %%%%%%%%%%%%%%%%%%%%%%%%%%%%%%%%%%%%%%%%%%%%%%%
% % if you get an error about newblock being undefined, uncomment this line:
% %\newcommand{\newblock}{}





% %Reference citation instructions and examples:
% %
% % Please use ONLY \cite and \citeA for reference citations.
% % \cite for parenthetical references
% % ...as shown in recent studies (Simpson et al., 2019)
% % \citeA for in-text citations
% % ...Simpson et al (2019) have shown...
% % DO NOT use other cite commands (e.g., \citet, \citep, \citeyear, \nocite, \citealp, etc.).
% %
% %
% %...as shown by \citeA{jskilby}.
% %...as shown by \citeA{lewin76}, \citeA{carson86}, \citeA{bartoldy02}, and \citeA{rinaldi03}.
% %...has been shown \cite<e.g.,>{jskilbye}.
% %...has been shown \cite{lewin76,carson86,bartoldy02,rinaldi03}.
% %...has been shown \cite{lewin76,carson86,bartoldy02,rinaldi03}.
% %
% % apacite uses < > for prenotes, not [ ]
% % DO NOT use other cite commands (e.g., \citet, \citep, \citeyear, \nocite, \citealp, etc.).
% %

% %% ------------------------------------------------------------------------ %%
% %
% %  END ARTICLE
% %
% %% ------------------------------------------------------------------------ %%

% \end{article}

% % Copy/paste for multiples of each file type as needed.

% % enter figures and tables below here: %%%%%%%
% %
% %
% %
% %
% % EXAMPLE FIGURES
% % ---------------
% % If you get an error about an unknown bounding box, try specifying the width and height of the figure with the natwidth and natheight options.
% % \begin{figure}
% %\setfigurenum{S1} %%You can change number for each figure if you want, not required. "S" prepended automatically.
% % \noindent\includegraphics[natwidth=800px,natheight=600px]{samplefigure.eps}
% %\caption{caption}
% %\label{epsfiguresample}
% %\end{figure}
% %
% %
% % Giving latex a width will help it to scale the figure properly. A simple trick is to use \textwidth. Try this if large figures run off the side of the page.
% % \begin{figure}
% % \noindent\includegraphics[width=\textwidth]{anothersample.png}
% %\caption{caption}
% %\label{pngfiguresample}
% %\end{figure}
% %
% %
% %\begin{figure}
% %\noindent\includegraphics[width=\textwidth]{athirdsample.pdf}
% %\caption{A pdf test figure}
% %\label{pdffiguresample}
% %\end{figure}
% %
% % PDFLatex does not seem to be able to process EPS figures. You may want to try the epstopdf package.
% %
% %
% % ---------------
% % EXAMPLE TABLE
% %a
% %\begin{table}
% %\settablenum{S1} %%Change number for each table
% %\caption{Time of the Transition Between Phase 1 and Phase 2\tablenotemark{a}}
% %\centering
% %\begin{tabular}{l c}
% %\hline
% % Run  & Time (min)  \\
% %\hline
% %  $l1$  & 260   \\
% %  $l2$  & 300   \\
% %  $l3$  & 340   \\
% %  $h1$  & 270   \\
% %  $h2$  & 250   \\
% %  $h3$  & 380   \\
% %  $r1$  & 370   \\
% %  $r2$  & 390   \\
% %\hline
% %\end{tabular}
% %\tablenotetext{a}{Footnote text here.}
% %\end{table}
% % ---------------
% %
% % EXAMPLE LARGE TABLE (UPLOADED SEPARATELY)
% %\begin{table}
% %\settablenum{S1} %%Change number for each table
% %\caption{Time of the Transition Between Phase 1 and Phase 2\tablenotemark{a}}
% %\end{table}


% \end{document}

% %%%%%%%%%%%%%%%%%%%%%%%%%%%%%%%%%%%%%%%%%%%%%%%%%%%%%%%%%%%%%%%

% More Information and Advice:

% %% ------------------------------------------------------------------------ %%
% %
% %  SECTION HEADS
% %
% %% ------------------------------------------------------------------------ %%

% % Capitalize the first letter of each word (except for
% % prepositions, conjunctions, and articles that are
% % three or fewer letters).

% % AGU follows standard outline style; therefore, there cannot be a section 1 without
% % a section 2, or a section 2.3.1 without a section 2.3.2.
% % Please make sure your section numbers are balanced.
% % ---------------
% % Level 1 head
% %
% % Use the \section{} command to identify level 1 heads;
% % type the appropriate head wording between the curly
% % brackets, as shown below.
% %
% %An example:
% %\section{Level 1 Head: Introduction}
% %
% % ---------------
% % Level 2 head
% %
% % Use the \subsection{} command to identify level 2 heads.
% %An example:
% %\subsection{Level 2 Head}
% %
% % ---------------
% % Level 3 head
% %
% % Use the \subsubsection{} command to identify level 3 heads
% %An example:
% %\subsubsection{Level 3 Head}
% %
% %---------------
% % Level 4 head
% %
% % Use the \subsubsubsection{} command to identify level 3 heads
% % An example:
% %\subsubsubsection{Level 4 Head} An example.
% %
% %% ------------------------------------------------------------------------ %%
% %
% %  IN-TEXT LISTS
% %
% %% ------------------------------------------------------------------------ %%
% %
% % Do not use bulleted lists; enumerated lists are okay.
% % \begin{enumerate}
% % \item
% % \item
% % \item
% % \end{enumerate}
% %
% %% ------------------------------------------------------------------------ %%
% %
% %  EQUATIONS
% %
% %% ------------------------------------------------------------------------ %%

% % Single-line equations are centered.
% % Equation arrays will appear left-aligned.

% Math coded inside display math mode \[ ...\]
%  will not be numbered, e.g.,:
%  \[ x^2=y^2 + z^2\]

%  Math coded inside \begin{equation} and \end{equation} will
%  be automatically numbered, e.g.,:
%  \begin{equation}
%  x^2=y^2 + z^2
%  \end{equation}

% % IF YOU HAVE MULTI-LINE EQUATIONS, PLEASE
% % BREAK THE EQUATIONS INTO TWO OR MORE LINES
% % OF SINGLE COLUMN WIDTH (20 pc, 8.3 cm)
% % using double backslashes (\\).

% % To create multiline equations, use the
% % \begin{eqnarray} and \end{eqnarray} environment
% % as demonstrated below.
% \begin{eqnarray}
%   x_{1} & = & (x - x_{0}) \cos \Theta \nonumber \\
%         && + (y - y_{0}) \sin \Theta  \nonumber \\
%   y_{1} & = & -(x - x_{0}) \sin \Theta \nonumber \\
%         && + (y - y_{0}) \cos \Theta.
% \end{eqnarray}

% %If you don't want an equation number, use the star form:
% %\begin{eqnarray*}...\end{eqnarray*}

% % Break each line at a sign of operation
% % (+, -, etc.) if possible, with the sign of operation
% % on the new line.

% % Indent second and subsequent lines to align with
% % the first character following the equal sign on the
% % first line.

% % Use an \hspace{} command to insert horizontal space
% % into your equation if necessary. Place an appropriate
% % unit of measure between the curly braces, e.g.
% % \hspace{1in}; you may have to experiment to achieve
% % the correct amount of space.


% %% ------------------------------------------------------------------------ %%
% %
% %  EQUATION NUMBERING: COUNTER
% %
% %% ------------------------------------------------------------------------ %%

% % You may change equation numbering by resetting
% % the equation counter or by explicitly numbering
% % an equation.

% % To explicitly number an equation, type \eqnum{}
% % (with the desired number between the brackets)
% % after the \begin{equation} or \begin{eqnarray}
% % command.  The \eqnum{} command will affect only
% % the equation it appears with; LaTeX will number
% % any equations appearing later in the manuscript
% % according to the equation counter.
% %

% % If you have a multiline equation that needs only
% % one equation number, use a \nonumber command in
% % front of the double backslashes (\\) as shown in
% % the multiline equation above.

% %% ------------------------------------------------------------------------ %%
% %
% %  SIDEWAYS FIGURE AND TABLE EXAMPLES
% %
% %% ------------------------------------------------------------------------ %%
% %
% % For tables and figures, add \usepackage{rotating} to the paper and add the rotating.sty file to the folder.
% % AGU prefers the use of {sidewaystable} over {landscapetable} as it causes fewer problems.
% %
% % \begin{sidewaysfigure}
% % \includegraphics[width=20pc]{samplefigure.eps}
% % \caption{caption here}
% % \label{label_here}
% % \end{sidewaysfigure}
% %
% %
% %
% % \begin{sidewaystable}
% % \caption{}
% % \begin{tabular}
% % Table layout here.
% % \end{tabular}
% % \end{sidewaystable}
% %
% %
